# Supplementary material for: Demand-Driven Pointer Analysis with Strong Updates via Value-Flow Refinement
Source: arXiv:1701.05650 source file (2017-01-20)
Supplement: Supplementary file 1 [file 8.appendix.tex]

% !TEX root =  fse16.tex

\clearpage
\newpage

\setcounter{figure}{0}
\setcounter{table}{0}

\onecolumn

\section{More Experimental Results}

\vspace*{2cm}
\begin{table*}[!h]
	\begin{center}
		\begin{tabular}{|c|r|r|r|r|r|}
			\hline
			\multirow{2}{*}{Program} & \multicolumn{4}{c|}{Pre-Processing Time of Pre-Analysis Shared by \vfsu and \SFS} & \multicolumn{1}{c|}{\multirow{2}{*}{Analysis Time of \SFS}} \\ \cline{2-5}
			 & \multicolumn{1}{c|}{Andersen's Analysis} & \multicolumn{1}{c|}{MemSSA} & \multicolumn{1}{c|}{SVFG} & \multicolumn{1}{c|}{Total} & \\ \hline \hline
			 milc & 0.42 & 0.03 & 0.07 & 0.52 & 0.16 \\ \hline
			 less & 0.42 & 0.14 & 0.23 & 0.79 & 1.94 \\ \hline
			 hmmer & 1.57 & 0.17 & 0.29 & 2.03 & 1.07 \\ \hline
			 make & 1.74 & 0.47 & 0.7 & 2.91 & 13.94 \\ \hline
			 a2ps & 7.34 & 0.51 & 0.8 & 8.65 & 60.61 \\ \hline
			 bison & 8.18 & 1.48 & 2.18 & 11.84 & 44.16 \\ \hline
			 grep & 1.44 & 0.06 & 0.11 & 1.61 & 2.39 \\ \hline
			 tar & 2.73 & 0.59 & 1.12 & 4.44 & 12.27 \\ \hline
			 bash & 53.48 & 20.4 & 23.67 & 97.55 & 2590.69 \\ \hline
			 sendmail & 24.05 & 9.74 & 13.69 & 47.48 & 348.63 \\ \hline
			 vim & 445.88 & 38.37 & 47.32 & 531.57 & 13823.00 \\ \hline
			 emacs & 135.93 & 61.11 & 85.83 & 282.87 & 8047.55 \\ \hline
		 \end{tabular}
	 \end{center}
\caption{Pre-processing times taken by pre-analysis shared by
	\vfsu and \SFS and analysis times of \SFS (in seconds) \label{fig:pre-analysis}}
\end{table*}

\vspace*{2cm}

\begin{table*}[h]
\begin{center}
\scalebox{0.83}{
\begin{tabular}{|c|c|c|c|c|c|c|c|c|c|c|c|c|c|c|c|}
\hline

Program & \multicolumn{15}{c|}{Budget} \\ \cline{2-16}
 & 0 & 10 & 20 & 40 & 100 & 200 & 400 & 1000 & 2000 & 4000 & 10000 & 20000 & 40000 & 100000 & 200000 \\ \hline

milc & 0 & 13 & 16 & 16 & 16 & 16 & 16 & 16 & 16 & 16 & 16 & 16 & 16 & 16 & 16 \\ \hline
less & 0 & 74 & 91 & 121 & 161 & 183 & 212 & 229 & 233 & 263 & 264 & 266 & 266 & 266 & 266 \\ \hline
hmmer & 0 & 77 & 149 & 168 & 178 & 185 & 189 & 190 & 190 & 190 & 192 & 192 & 192 & 192 & 192 \\ \hline
make & 0 & 27 & 43 & 61 & 85 & 98 & 107 & 129 & 141 & 148 & 148 & 148 & 149 & 171 & 170 \\ \hline
a2ps & 0 & 685 & 759 & 834 & 954 & 972 & 969 & 977 & 1041 & 1111 & 1111 & 1130 & 1130 & 996 & 1165 \\ \hline
bison & 0 & 550 & 823 & 907 & 969 & 1005 & 1011 & 1028 & 1119 & 1114 & 1272 & 1321 & 1331 & 1330 & 1422 \\ \hline
grep & 0 & 72 & 97 & 110 & 129 & 167 & 172 & 172 & 172 & 172 & 173 & 179 & 179 & 179 & 179 \\ \hline
tar & 0 & 173 & 262 & 334 & 372 & 407 & 418 & 503 & 515 & 523 & 522 & 529 & 527 & 543 & 543 \\ \hline
bash & 0 & 163 & 192 & 211 & 218 & 230 & 235 & 242 & 242 & 246 & 258 & 277 & 305 & 358 & 554 \\ \hline
sendmail & 0 & 188 & 362 & 471 & 523 & 559 & 615 & 644 & 641 & 670 & 669 & 673 & 683 & 691 & 707 \\ \hline
vim & 0 & 250 & 342 & 425 & 532 & 620 & 728 & 1148 & 1492 & 1204 & 1620 & 1581 & 1797 & 2309 & 2427 \\ \hline
emacs & 0 & 152 & 201 & 225 & 309 & 326 & 338 & 351 & 359 & 394 & 448 & 588 & 742 & 1243 & 1662 \\ \hline
\end{tabular}
}
\end{center}
\caption{Number of strong updates performed by \vfsu under 
different budgets
\label{tab:su}
}
\end{table*}

\begin{table*}[ht]
\begin{center}
\scalebox{0.83}{
\begin{tabular}{|c|c|c|c|c|c|c|c|c|c|c|c|c|c|c|c|c|}
\hline

& \multicolumn{15}{c|}{\vfsu} & \multicolumn{1}{c|}{ \multirow{3}{*}{\SFS}} \\ \cline{2-16}
Program & \multicolumn{15}{c|}{Budget} & \multirow{2}{*}{} \\ \cline{2-16}
 & 0 & 10 & 20 & 40 & 100 & 200 & 400 & 1000 & 2000 & 4000 & 10000 & 20000 & 40000 & 100000 & 200000 & \\ \hline

milc & 3 & 3 & 3 & 3 & 3 & 3 & 3 & 3 & 3 & 3 & 3 & 3 & 3 & 3 & 3 & 3 \\ \hline
less & 53 & 53 & 52 & 52 & 52 & 52 & 51 & 51 & 50 & 50 & 37 & 13 & 13 & 13 & 12 & 12 \\ \hline
hmmer & 117 & 115 & 108 & 106 & 106 & 105 & 105 & 87 & 87 & 87 & 86 & 86 & 86 & 86 & 86 & 86 \\ \hline
make & 35 & 33 & 33 & 33 & 33 & 33 & 26 & 26 & 26 & 26 & 26 & 26 & 26 & 23 & 23 & 23 \\ \hline
a2ps & 55 & 55 & 46 & 45 & 39 & 36 & 35 & 34 & 34 & 34 & 34 & 24 & 24 & 24 & 12 & 12 \\ \hline
bison & 103 & 102 & 98 & 97 & 95 & 94 & 94 & 94 & 94 & 94 & 94 & 94 & 94 & 94 & 63 & 63 \\ \hline
grep & 27 & 25 & 19 & 17 & 17 & 17 & 14 & 14 & 14 & 14 & 14 & 13 & 13 & 13 & 13 & 11 \\ \hline
tar & 90 & 88 & 82 & 78 & 75 & 74 & 73 & 71 & 71 & 70 & 70 & 70 & 70 & 62 & 62 & 62 \\ \hline
bash & 23 & 19 & 18 & 18 & 18 & 18 & 17 & 17 & 17 & 17 & 17 & 17 & 17 & 17 & 17 & 17 \\ \hline
sendmail & 134 & 129 & 127 & 124 & 116 & 115 & 115 & 108 & 108 & 94 & 94 & 94 & 94 & 94 & 94 & 94 \\ \hline
vim & 261 & 234 & 230 & 225 & 220 & 220 & 218 & 218 & 218 & 218 & 218 & 218 & 218 & 218 & 218 & 218 \\ \hline
emacs & 71 & 56 & 52 & 50 & 47 & 47 & 46 & 46 & 46 & 46 & 45 & 45 & 45 & 45 & 45 & 45 \\ \hline
\end{tabular}
}
\end{center}
\caption{Number of \ato's reported by both \vfsu under
	different budgets and \SFS 
	\label{fig:uninitobj}
}
\end{table*}
